# Supplementary material for: Geometry, electronic structure, and optical properties of boron cages: A first-principles DFT study
Source: arXiv:2512.20114 source file (2025-12-23)
Supplement: Supplementary file 1 [file Supporting_Information.pdf]

# Supporting Information

## Geometry, electronic structure, and optical properties of boron cages: A first-principles DFT study

Kashinath T. Chavan[1], Ihsan Boustani[2], and Alok Shukla[1]

[1]*Department of Physics, Indian Institute of Technology Bombay, Mumbai 400076, India.*

[2]*Theoretical and Computational Chemistry, Faculty of Mathematics and Natural Sciences, Bergische Universität Wuppertal, D-42097 Wuppertal, Germany*

---------------

Oscillator strengths and wavefunctions corresponding to largest coefficient of excitations in Boron cage clusters.

## 1. $B_{20}$ ($D_{5h}$)

| Peak | Energy (eV) | OS | Wave function |
|---|---|---|---|
| I | 1.169 | 0.0031 | H:L+1 |
| II | 1.5814 | 0.0014 | H-1:L+1 |
| | 1.7861 | 0.0019 | H-4:L |
| | 1.8333 | 0.0047 | H-2:L |
| III | 2.2142 | 0.0025 | H-2:L+1 |
| | 2.2513 | 0.0021 | H-5:L+1 |
| IV | 2.6692 | 0.0596 | H-2:L+1 |
| | 2.6727 | 0.0075 | H:L+2 |
| V | 2.9748 | 0.0143 | H-6:L+1 |
| | 3.2661 | 0.0498 | H-1:L+2 |
| | 3.3704 | 0.0209 | H-8:L+1 |
| | 3.4887 | 0.0595 | H:L+5 |
| | 3.5273 | 0.0410 | H:L+5 |
| | 3.7543 | 0.0172 | H-3:L+3 |
| | 3.8615 | 0.0403 | H-4:L+3 |

## 2. $B_{20}$ (Dodecahedron)

| Peak | Energy (eV) | OS | Wave function |
|---|---|---|---|

| | | | |
|---|---|---|---|
| I | 2.2645 | 0.0065 | H-4:L |
| | 2.2939 | 0.0147 | H-4:L+1 |
| II | 3.0165 | 0.0023 | H-1:L+3 |
| | 3.0430 | 0.0106 | H-3:L+4 |
| III | 3.7937 | 0.3196 | H:L+5 |

# 3. $B_{32}$

| Peak | Energy (eV) | OS | Wave function |
|---|---|---|---|
| I | 2.5953 | 0.0163 | H-1:L+3 |
| | 2.5963 | 0.0164 | H-2:L+3 |
| | 2.5966 | 0.0164 | H-2:L+4 |

# 4. $B_{42}$

| Peak | Energy (eV) | OS | Wave function |
|---|---|---|---|
| I | 1.3164 | 0.0022 | H:L |
| | 1.4240 | 0.0039 | H-1:L |
| II | 2.0928 | 0.0063 | H-1:L+2 |
| | 2.1549 | 0.0018 | H-2:L+2 |
| III | 2.4337 | 0.0034 | H-5:L |
| | 2.4856 | 0.0055 | H-1:L+5 |
| IV | 2.6277 | 0.0037 | H-1:L+6 |
| | 2.6527 | 0.0033 | H-5:L+1 |
| | 2.7032 | 0.0035 | H-2:L+2 |
| | 2.7609 | 0.0055 | H:L+7 |
| | 2.8176 | 0.0034 | H-1:L+7 |
| | 2.9111 | 0.0081 | H-3:L+3 |
| | 2.9703 | 0.0061 | H-8:L |
| | 2.9929 | 0.0032 | H:L+8 |
| | 3.0012 | 0.0047 | H-4:L+2 |
| V | 3.1123 | 0.0037 | H-5:L+1 |
| | 3.1563 | 0.0062 | H-3:L+5 |
| | 3.1654 | 0.0045 | H-1:L+9 |
| | 3.2083 | 0.0044 | H-4:L+3 |
| | 3.2330 | 0.0039 | H:L+10 |
| | 3.3083 | 0.0058 | H-10:L |
| | 3.3285 | 0.0055 | H-1:L+10 |
| | 3.3742 | 0.0044 | H-4:L+4 |
| | 3.4326 | 0.0049 | H-1:L+11 |
| | 3.4588 | 0.0097 | H-5:L+4 |
| | 3.4765 | 0.0123 | H-3:L+7 |

| | | | |
|---|---|---|---|
| | 3.5145 | 0.0048 | H-2:L+11 |
| VI | 3.8207<br>3.8310<br>3.8467<br>3.8803<br>3.8900<br>3.8958<br>3.9187<br>3.9312<br>3.9448 | 0.0047<br>0.0120<br>0.0081<br>0.0046<br>0.0067<br>0.0064<br>0.0027<br>0.0075<br>0.0027 | H:L+14<br>H:L+13<br>H-3:L+9<br>H-8:L+3<br>H-7:L+4<br>H-1:L+13<br>H-1:L+14<br>H-1:L+14<br>H-9:L+2 |
| VII | 3.9630<br>3.9695<br>3.9799<br>3.9847<br>4.0037<br>4.0097 | 0.0057<br>0.0022<br>0.0062<br>0.0063<br>0.0064<br>0.0107 | H-4:L+8<br>H-2:L+13<br>H-2:L+13<br>H-4:L+8<br>H-6:L+7<br>H-2:L+14 |

# 5. $B_{60}$

| Peak | Energy (eV) | OS | Wave function |
|---|---|---|---|
| I | 1.2632<br>1.4624<br>1.5633 | 0.0037<br>0.0029<br>0.0164 | H-2:L<br>H-4:L<br>H-2:L+2 |
| II | 1.8151<br>1.8451<br>2.0052 | 0.0109<br>0.0092<br>0.0053 | H-2:L+3<br>H-4:L+2<br>H-4:L+3 |
| III | 2.1232<br>2.1750<br>2.2082<br>2.2353<br>2.3377<br>2.4155<br>2.4420<br>2.5099<br>2.5315<br>2.5927<br>2.6842<br>2.7297<br>2.7669 | 0.0055<br>0.0048<br>0.0039<br>0.0059<br>0.0081<br>0.0089<br>0.0085<br>0.0117<br>0.0096<br>0.0127<br>0.0051<br>0.0044<br>0.0071 | H:L+5<br>H-7:L<br>H-1:L+3<br>H-2:L+4<br>H:L+6<br>H-3:L+3<br>H-7:L+1<br>H-3:L+5<br>H-1:L+6<br>H:L+8<br>H-3:L+6<br>H-10:L<br>H-10:L |

# 6. $B_{72}$

| Peak | Energy (eV) | OS | Wave function |
|---|---|---|---|
| I | 0.52467 | 0.0028 | H-2:L |
| | 0.52945 | 0.0030 | H-2:L+1 |
| | 0.78933 | 0.0069 | H-5:L |
| | 0.81205 | 0.0058 | H-4:L+2 |
| | 0.81246 | 0.0056 | H-5:L+2 |
| II | 1.27488 | 0.0039 | H-3:L+5 |
| | 1.27568 | 0.0037 | H-3:L+6 |
| | 1.32940 | 0.0265 | H-2:L+4 |
| | 1.43608 | 0.0034 | H-4:L+3 |
| | 1.43626 | 0.0030 | H-5:L+3 |
| | 1.53923 | 0.0187 | H-4:L+4 |
| | 1.54107 | 0.0179 | H-5:L+5 |
| | 1.58052 | 0.0087 | H-5:L+5 |
| | 1.76986 | 0.0043 | H-1:L+7 |
| | 1.77269 | 0.0043 | H-1:L+10 |

## 7. $B_{80}$

| Peak | Energy (eV) | OS | Wave function |
|---|---|---|---|
| I | 1.9906 | 0.0271 | H-4:L+3 |

## 8. $B_{92}$

| Peak | Energy (eV) | OS | Wave function |
|---|---|---|---|
| I | 0.84647 | 0.0211 | H-3:L |
| | 0.95337 | 0.0071 | H-5:L |
| | 1.2238 | 0.0073 | H:L+1 |
| II | 1.78051 | 0.0165 | H-2:L+6 |
| | 1.80118 | 0.0139 | H-3:L+6 |
| | 1.841714 | 0.0096 | H-4:L+3 |
| | 1.971539 | 0.0042 | H-4:L+5 |

## 9. $B_{92}$ (Icosahedron)

| Peak | Energy (eV) | OS | Wave function |
|---|---|---|---|
| I | 1.60202 | 0.0352 | H-2:L |
| | 1.6020 | 0.0352 | H-1:L+1 |
| | 1.6020 | 0.0354 | H:L+3 |

## 10. $B_{100}$

| Peak | Energy (eV) | OS | Wave function |
|---|---|---|---|

| | | | |
|---|---|---|---|
| I | 0.76801 | 0.0022 | H-4:L+3 |
| | 0.76977 | 0.0018 | H-4:L+3 |
| | 0.946813 | 0.0121 | H:L+4 |
| | 0.962415 | 0.0089 | H:L+4 |
| | 1.28704 | 0.0036 | H-1:L+5 |
| | 1.30977 | 0.0025 | H-2:L+5 |
| | 1.40861 | 0.0046 | H-10:L+3 |

# 11. B110 (Icosahedron)

| Peak | Energy (eV) | OS | Wave function |
|---|---|---|---|
| I | 0.891260 | 0.0022 | H:L+3 |
| | 0.898189 | 0.0061 | H:L+4 |
| | 0.900269 | 0.0061 | H-1:L+4 |
| | 1.147906 | 0.0037 | H-1:L+6 |
| | 1.148597 | 0.0038 | H-1:L+5 |
| | 1.375477 | 0.0114 | H-1:L+9 |

# 12. $B_{122}$

| **Peak** | **Energy (eV)** | **OS** | **Wave function** |
|---|---|---|---|
| I | 0.8744767282 | 0.0032 | H:L+3 |
| | 0.9134619097 | 0.0024 | H:L+4 |
| | 0.915079969 | 0.0024 | H-5:L |
| | 0.9750327149 | 0.0022 | H-6:L |
| | 1.025883572 | 0.0043 | H:L+5 |
| | 1.097341131 | 0.004 | H-3:L+1 |
| | 1.111248207 | 0.0041 | H-4:L+1 |
| | 1.161879721 | 0.0025 | H:L+6 |
| | 1.238529009 | 0.0030 | H-2:L+4 |
| | 1.244621195 | 0.0046 | H-6:L+1 |
| | 1.352328538 | 0.0023 | H-6:L+2 |
| | 1.357585216 | 0.0047 | H-6:L+3 |
| | 1.39697342 | 0.0038 | H-3:L+5 |
| | 1.421478354 | 0.0020 | H-5:L+4 |
| | 1.429113664 | 0.0030 | H-9:L |
| | 1.435267932 | 0.0031 | H-6:L+4 |
| | 1.466695669 | 0.0039 | H-10:L |
| | 1.505082547 | 0.0036 | H-7:L+1 |
| | 1.510491764 | 0.0030 | H-5:L+5 |

| | | | |
|---|---|---|---|
| | 1.533281207 | 0.0021 | H-6:L+5 |
| | 1.565160449 | 0.0043 | H-4:L+6 |
| | 1.582238196 | 0.0034 | H-11:L |
| | 1.603623941 | 0.0020 | H:L+9 |
| | 1.628585118 | 0.0034 | H-7:L+3 |
